# Supplementary material for: Empowering AIOps: Leveraging Large Language Models for IT Operations Management
Source: arXiv:2501.12461 source file (2025-01-23)
Supplement: Supplementary file 1 [file appendix.tex]

\onecolumn
%\begin{landscape}
\section{Appendix - Research Question Detailed Results}

\subsection{RQ1 - Detailed Summary}

\begin{longtable}[c]{| c | c | c | c | c | c | c | c | c | c | c |}    
    \caption{RQ1 - Large Language Model Agents solving task accuracy in AIOps Context.\label{tab:aiops-rq1-results}}\\
    \hline
    Query & Claude  & Claude & Claude & Mistral & Mixtral & Mistral & GPT & GPT & GPT & GPT\\
    No. & 3.5 & 3 & 3 & Largest &  8x22B & Small & 3.5 & 4-o & 4-o & 4 \\
    & Sonnet & Haiku & Opus & & & 7B & turbo & & mini & turbo\\
    \hline
    \endfirsthead
    \hline
    Query & Claude  & Claude & Claude & Mistral & Mixtral & Mistral & GPT & GPT & GPT & GPT\\
    No. & 3.5 & 3 & 3 & Largest &  8x22B & Small & 3.5 & 4-o & 4-o & 4 \\
    & Sonnet & Haiku & Opus & & & 7B & turbo & & mini & turbo\\
    \hline
    \endhead    
    \hline
    \endfoot    
    \hline
    \endlastfoot
    
    Q-01 & 100\% & 100\% & 100\% & 100\% & 100\% & 100\% & 100\% & 100\% & 100\% & 100\% \\
    \hline
    Q-02 & 100\% & 90\% & 100\% & 100\% & 100\% & 100\% & 100\% & 100\% & 100\% & 100\% \\
    \hline
    Q-03 & 100\% & 100\% & 100\% & 100\% & 100\% & 100\% & 100\% & 100\% & 100\% & 100\% \\
    \hline
    Q-04 & 100\% & 100\% & 100\% & 100\% & 100\% & 100\% & 0\% & 100\% & 100\% & 100\% \\ 
    \hline
    Q-05 & 100\% & 90\% & 100\% & 100\% & 0\% & 100\% & 100\% & 100\% & 100\% & 100\% \\
    \hline
    Q-06 & 100\% & 100\% & 100\% & 100\% & 0\% & 100\% & 100\% & 100\% & 100\% & 100\% \\
    \hline
    Q-07 & 100\% & 0\% & 0\% & 90\% & 0\% & 0\% & 100\% & 30\% & 0\% & 0\% \\
    \hline
    Q-08 & 100\% & 100\% & 100\% & 100\% & 100\% & 100\% & 100\% & 100\% & 100\% & 100\% \\
    \hline
    Q-09 & 0\% & 0\% & 0\% & 0\% & 0\% & 0\% & 0\% & 0\% & 0\% & 0\% \\
    \hline
    Q-10 & 100\% & 100\% & 100\% & 100\% & 0\% & 100\% & 100\% & 100\% & 100\% & 100\% \\
    \hline
    Q-11 & 100\% & 100\% & 100\% & 100\% & 0\% & 100\% & 100\% & 100\% & 100\% & 100\% \\ 
    \hline
    Q-12 & 100\% & 100\% & 100\% & 100\% & 0\% & 100\% & 100\% & 100\% & 100\% & 100\% \\
    \hline
    Q-13 & 100\% & 100\% & 100\% & 100\% & 0\% & 100\% & 100\% & 100\% & 100\% & 100\% \\
    \hline
    Q-14 & 100\% & 100\% & 100\% & 100\% & 0\% & 0\% & 100\% & 0\% & 0\% & 0\% \\
    \hline
    Q-15 & 100\% & 100\% & 100\% & 100\% & 0\% & 0\% & 100\% & 100\% & 100\% & 100\% \\
    \hline
    Q-16 & 100\% & 100\% & 100\% & 100\% & 0\% & 100\% & 100\% & 100\% & 100\% & 100\% \\
    \hline
    Q-17 & 100\% & 100\% & 100\% & 100\% & 0\% & 100\% & 100\% & 100\% & 100\% & 100\% \\
    \hline
    Q-18 & 100\% & 100\% & 100\% & 100\% & 0\% & 100\% & 100\% & 100\% & 100\% & 100\% \\
    \hline
    Q-19 & 100\% & 100\% & 100\% & 100\% & 0\% & 100\% & 100\% & 100\% & 100\% & 100\% \\
    \hline
    Q-20 & 100\% & 100\% & 100\% & 100\% & 0\% & 0\% & 0\% & 100\% & 100\% & 100\% \\
    \hline
    Q-21 & 80\% & 10\% & 0\% & 0\% & 0\% & 0\% & 0\% & 100\% & 100\% & 100\% \\
    \hline
    Q-22 & 100\% & 50\% & 100\% & 100\% & 0\% & 0\% & 0\% & 100\% & 100\% & 100\% \\
    \hline
    Q-23 & 100\% & 100\% & 90\% & 100\% & 0\% & 100\% & 100\% & 100\% & 100\% & 100\% \\
    \hline
    Q-24 & 100\% & 30\% & 100\% & 80\% & 0\% & 0\% & 0\% & 100\% & 100\% & 80\% \\
    \hline
    Q-25 & 100\%* & 30\%* & 100\%* & 0\% & 0\% & 0\% & 0\% & 100\% & 10\% & 80\% \\
\end{longtable}

\subsection{RQ2 - Detailed Summary}
\begin{longtable}[c]{| c | c | c | c | c | c | c | c | c | c | c | c |}    
    \caption{RQ2 - Large Language Model Agents solving task response times (in seconds) in AIOps Context.\label{tab:aiops-rq2-results}}\\
    \hline
    Query & Metric & Claude  & Claude & Claude & Mistral & Mixtral & Mistral & GPT & GPT & GPT & GPT\\
    No. & & 3.5 & 3 & 3 & Largest &  8x22B & Small & 3.5 & 4-o & 4-o & 4 \\
    & & Sonnet & Haiku & Opus & & & 7B & turbo & & mini & turbo \\
    \hline
    \endfirsthead
    \hline
    Query & Metric & Claude  & Claude & Claude & Mistral & Mixtral & Mistral & GPT & GPT & GPT & GPT\\
    No. & & 3.5 & 3 & 3 & Largest &  8x22B & Small & 3.5 & 4-o & 4-o & 4 \\
    & & Sonnet & Haiku & Opus & & & 7B & turbo & & mini & turbo \\
    \hline
    \endhead    
    \hline
    \endfoot
    \hline
    \endlastfoot
    
    & P-50 & 1.81 & 0.77 & 7.07 & 1.16 & 2.06 & 1.38 & 0.71 & 0.87 & 0.93 & 1.85 \\
    Q-01 & P-90 & 2.04 & 1.22 & 9.50 & 1.62 & 2.34 & 1.70 & 0.87 & 1.29 & 1.20 & 2.54 \\    
    & Max & 2.07 & 2.16 & 12.97 & 2.07 & 2.77 & 2.23 & 1.18 & 3.13 & 1.23 & 2.73 \\
    \hline
    & P-50 & 6.39 & 2.81 & 23.05 & 8.38 & 7.56 & 6.32 & 2.02 & 5.15 & 3.68 & 13.33 \\
    Q-02 & P-90 & 6.72 & 4.45 & 31.52 & 12.32 & 7.82 & 6.76 & 2.57 & 5.95 & 6.44 & 16.86 \\    
    & Max & 6.83 & 4.94 & 39.60 & 18.01 & 7.87 & 7.03 & 3.13 & 8.07 & 14.86 & 17.72 \\
    \hline
    & P-50 & 3.86 & 2.79 & 20.63 & 11.10 & 5.17 & 2.72 & 2.06 & 4.77 & 4.40 & 10.96 \\
    Q-03 & P-90 & 6.22 & 5.28 & 27.50 & 27.96 & 5.82 & 2.95 & 2.38 & 5.67 & 6.39 & 12.56 \\    
    & Max & 6.35 & 6.84 & 28.23 & 42.01 & 6.22 & 3.26 & 2.44 & 6.00 & 9.74 & 12.64 \\
    \hline
    & P-50 & 7.00 & 4.13 & 24.35 & 25.17 & 7.97 & 6.21 & 1.64 & 8.39 & 5.48 & 14.84 \\ 
    Q-04 & P-90 & 8.46 & 4.97 & 27.31 & 33.17 & 8.24 & 6.96 & 1.91 & 10.49 & 10.80 & 16.30 \\    
    & Max & 9.03 & 7.47 & 33.90 & 34.49 & 8.26 & 7.18 & 1.95 & 15.49 & 43.94 & 19.60 \\
    \hline
    & P-50 & 5.99 & 2.9 & 17.73 & 5.31 & 2.29 & 6.42 & 3.77 & 5.47 & 4.08 & 12.63 \\
    Q-05 & P-90 & 7.37 & 3.88 & 20.60 & 6.62 & 2.85 & 6.89 & 4.36 & 6.43 & 6.84 & 13.62 \\    
    & Max & 7.49 & 4.13 & 20.94 & 7.53 & 3.11 & 7.08 & 4.38 & 6.67 & 10.80 & 13.62 \\
    \hline
    & P-50 & 4.95 & 2.09 & 16.37 & 5.53 & 2.53 & 4.86 & 4.02 & 4.12 & 3.76 & 9.48 \\
    Q-06 & P-90 & 5.18 & 2.36 & 18.53 & 9.46 & 2.85 & 5.11 & 4.73 & 4.98 & 5.09 & 11.73 \\    
    & Max & 5.27 & 2.52 & 18.92 & 9.54 & 3.14 & 5.64 & 4.76 & 5.59 & 6.45 & 12.84 \\
    \hline
    & P-50 & 7.53 & 3.14 & 23.69 & 6.46 & 7.08 & 5.56 & 3.59 & 8.19 & 9.46 & 25.81 \\
    Q-07 & P-90 & 8.62 & 4.95 & 26.87 & 11.74 & 7.99 & 6.36 & 4.08 & 11.28 & 17.28 & 28.15 \\    
    & Max & 8.79 & 5.77 & 32.01 & 11.88 & 9.10 & 6.72 & 4.58 & 13.66 & 17.55 & 29.08 \\
    \hline
    & P-50 & 3.97 & 1.96 & 12.45 & 3.83 & 1.95 & 2.61 & 2.34 & 2.00 & 1.78 & 5.68 \\
    Q-08 & P-90 & 4.47 & 3.71 & 13.30 & 6.50 & 2.58 & 2.76 & 3.43 & 2.51 & 2.31 & 6.66 \\    
    & Max & 4.54 & 4.23 & 13.46 & 6.74 & 2.66 & 2.82 & 3.80 & 3.02 & 3.71 & 6.86 \\
    \hline
    & P-50 & 2.64 & 1.08 & 11.38 & 23.71 & 2.20 & 1.83 & 1.64 & 0.87 & 0.98 & 1.60 \\
    Q-09 & P-90 & 2.93 & 2.17 & 13.67 & 28.07 & 2.63 & 1.92 & 1.72 & 1.79 & 2.20 & 2.66 \\    
    & Max & 3.07 & 2.30 & 13.76 & 51.20 & 2.71 & 2.00 & 1.95 & 1.99 & 2.74 & 3.88 \\
    \hline
    & P-50 & 10.61 & 6.36 & 22.38 & 13.58 & 6.09 & 8.53 & 8.28 & 10.31 & 8.98 & 16.17 \\
    Q-10 & P-90 & 10.97 & 7.06 & 23.45 & 18.39 & 6.36 & 8.85 & 10.60 & 12.01 & 14.82 & 18.78 \\    
    & Max & 11.03 & 7.27 & 23.72 & 25.84 & 6.86 & 8.93 & 10.90 & 15.89 & 29.50 & 19.26 \\
    \hline
    & P-50 & 10.52 & 5.93 & 22.81 & 12.27 & 4.70 & 9.01 & 8.19 & 8.23 & 8.67 & 15.19 \\ 
    Q-11 & P-90 & 11.17 & 8.42 & 23.28 & 14.58 & 4.89 & 10.02 & 8.94 & 9.36 & 9.86 & 16.32 \\    
    & Max & 11.61 & 10.04 & 23.49 & 22.14 & 5.16 & 10.30 & 9.08 & 10.58 & 10.31 & 17.42 \\
    \hline
    & P-50 & 11.04 & 6.21 & 22.00 & 11.30 & 3.52 & 8.64 & 7.74 & 8.71 & 8.81 & 15.78 \\
    Q-12 & P-90 & 11.72 & 6.98 & 26.90 & 19.09 & 15.42 & 8.88 & 8.57 & 12.04 & 10.93 & 17.68 \\    
    & Max & 12.36 & 7.17 & 27.72 & 20.55 & 120.12 & 9.04 & 8.92 & 16.60 & 11.75 & 20.88 \\
    \hline
    & P-50 & 8.33 & 5.45 & 20.05 & 8.17 & 3.37 & 6.94 & 6.69 & 6.65 & 6.46 & 12.14 \\
    Q-13 & P-90 & 9.07 & 6.89 & 22.06 & 15.11 & 3.74 & 7.54 & 7.14 & 8.09 & 8.43 & 13.01 \\    
    & Max & 9.32 & 7.27 & 22.96 & 15.48 & 4.49 & 7.74 & 7.58 & 9.36 & 11.30 & 13.76 \\
    \hline
    & P-50 & 5.03 & 1.77 & 15.89 & 2.66 & 5.26 & 1.39 & 1.59 & 0.57 & 0.67 & 0.90 \\
    Q-14 & P-90 & 5.77 & 1.85 & 17.29 & 3.23 & 5.82 & 1.91 & 1.86 & 0.60 & 1.08 & 1.09 \\    
    & Max & 6.27 & 2.15 & 18.10 & 3.46 & 6.14 & 2.58 & 2.03 & 0.62 & 1.09 & 1.11 \\
    \hline
    & P-50 & 5.39 & 1.86 & 16.80 & 3.44 & 2.53 & 2.55 & 1.77 & 2.07 & 1.70 & 3.53 \\
    Q-15 & P-90 & 5.81 & 3.32 & 17.29 & 5.11 & 3.28 & 2.97 & 1.95 & 2.54 & 2.49 & 4.81 \\    
    & Max & 5.83 & 4.02 & 18.10 & 10.68 & 3.38 & 3.11 & 2.03 & 3.02 & 6.39 & 5.57 \\
    \hline
    & P-50 & 5.55 & 2.29 & 16.24 & 3.81 & 3.33 & 2.98 & 2.06 & 2.19 & 1.97 & 4.41 \\
    Q-16 & P-90 & 5.94 & 3.83 & 19.09 & 4.88 & 3.51 & 3.40 & 2.33 & 3.30 & 3.43 & 5.17 \\    
    & Max & 6.10 & 5.85 & 19.31 & 5.15 & 3.69 & 3.52 & 2.50 & 4.39 & 3.62 & 5.69 \\
    \hline
    & P-50 & 6.36 & 2.32 & 16.42 & 4.60 & 8.77 & 3.18 & 2.10 & 2.44 & 2.06 & 4.34 \\
    Q-17 & P-90 & 6.69 & 2.98 & 18.86 & 5.64 & 9.47 & 3.54 & 2.24 & 3.17 & 2.37 & 5.13 \\    
    & Max & 7.01 & 3.53 & 18.97 & 6.36 & 9.54 & 3.60 & 2.64 & 3.62 & 2.43 & 7.40 \\
    \hline
    & P-50 & 5.73 & 2.04 & 17.34 & 3.87 & 5.45 & 3.17 & 2.16 & 2.19 & 2.47 & 4.67 \\
    Q-18 & P-90 & 6.92 & 2.19 & 19.91 & 5.60 & 5.90 & 3.74 & 2.34 & 3.07 & 3.46 & 5.29 \\    
    & Max & 6.95 & 2.78 & 20.39 & 5.80 & 6.35 & 3.96 & 2.52 & 5.46 & 4.51 & 5.34 \\
    \hline
    & P-50 & 6.19 & 2.29 & 16.35 & 5.81 & 8.84 & 3.13 & 2.09 & 2.27 & 2.13 & 4.38 \\
    Q-19 & P-90 & 6.42 & 4.48 & 18.52 & 8.56 & 9.52 & 3.59 & 2.53 & 2.84 & 2.59 & 5.79 \\    
    & Max & 6.69 & 6.49 & 20.99 & 14.72 & 9.54 & 3.80 & 2.91 & 2.87 & 4.29 & 6.64 \\
    \hline
    & P-50 & 5.31 & 2.25 & 15.62 & 6.58 & 5.18 & 4.17 & 1.97 & 2.12 & 2.54 & 3.91 \\
    Q-20 & P-90 & 5.72 & 3.31 & 18.28 & 8.42 & 5.37 & 4.77 & 8.02 & 4.75 & 2.84 & 4.90 \\    
    & Max & 6.04 & 3.45 & 19.57 & 8.63 & 5.41 & 5.68 & 8.20 & 5.82 & 2.84 & 6.00 \\
    \hline
    & P-50 & 17.68 & 5.90 & 37.57 & 124.03 & 6.28 & 9.22 & 3.54 & 75.95 & 66.59 & 21.11 \\
    Q-21 & P-90 & 20.51 & 6.97 & 42.13 & 126.67 & 6.60 & 9.42 & 3.76 & 91.96 & 75.10 & 26.04 \\    
    & Max & 20.72 & 7.06 & 47.22 & 126.71 & 6.75 & 9.64 & 3.99 & 118.36 & 77.52 & 28.39 \\
    \hline
    & P-50 & 16.51 & 7.79 & 41.35 & 23.20 & 6.83 & 11.14 & 8.10 & 9.15 & 9.86 & 18.68 \\
    Q-22 & P-90 & 17.74 & 10.38 & 47.66 & 26.49 & 7.27 & 11.81 & 8.23 & 10.37 & 11.68 & 20.98 \\    
    & Max & 18.43 & 12.43 & 49.04 & 32.98 & 8.02 & 12.13 & 8.23 & 12.20 & 12.22 & 22.43 \\
    \hline
    & P-50 & 10.43 & 5.47 & 23.17 & 8.74 & 3.44 & 7.46 & 6.12 & 6.26 & 5.77 & 11.03 \\
    Q-23 & P-90 & 11.38 & 7.62 & 25.48 & 12.47 & 3.76 & 7.89 & 6.71 & 7.33 & 6.61 & 12.10 \\    
    & Max & 15.19 & 7.96 & 28.87 & 38.28 & 4.54 & 8.01 & 7.06 & 7.99 & 9.01 & 12.79 \\
    \hline
    & P-50 & 10.84 & 4.41 & 37.27 & 8.42 & 6.99 & 10.99 & 8.13 & 6.38 & 7.69 & 13.19 \\
    Q-24 & P-90 & 11.20 & 9.94 & 42.08 & 24.29 & 7.20 & 11.21 & 8.59 & 8.00 & 13.26 & 14.88 \\    
    & Max & 11.74 & 10.99 & 44.95 & 37.83 & 7.59 & 11.28 & 8.60 & 8.67 & 14.55 & 19.17 \\
    \hline
    & P-50 & 31.54 & 18.18 & 77.33 & 132.14 & 7.40 & 5.12 & 8.19 & 92.99 & 4.16 & 141.51 \\
    Q-25 & P-90 & 32.72 & 37.02 & 88.60 & 174.69 & 7.62 & 5.22 & 8.80 & 107.35 & 14.42 & 158.07 \\    
    & Max & 33.15 & 37.39 & 88.96 & 181.16 & 7.64 & 5.58 & 10.03 & 138.38 & 79.72 & 158.40 \\
\end{longtable}

\subsection{RQ3 - Detailed Summary}

\begin{longtable}[c]{| c | c | c | c | c | c | c | c | c | c | c |}    
    \caption{RQ3 - Average token count (verbosity) of Large Language Model Agents solving task in AIOps Context.\label{tab:aiops-rq3-results}}\\
    \hline
    Query & Claude  & Claude & Claude & Mistral & Mixtral & Mistral & GPT & GPT & GPT & GPT\\
    No. & 3.5 & 3 & 3 & Largest &  8x22B & Small & 3.5 & 4-o & 4-o & 4 \\
    & Sonnet & Haiku & Opus & & & 7B & turbo & & mini & turbo\\
    \hline
    \endfirsthead
    \hline
    Query & Claude  & Claude & Claude & Mistral & Mixtral & Mistral & GPT & GPT & GPT & GPT\\
    No. & 3.5 & 3 & 3 & Largest &  8x22B & Small & 3.5 & 4-o & 4-o & 4 \\
    & Sonnet & Haiku & Opus & & & 7B & turbo & & mini & turbo\\
    \hline
    \endhead    
    \hline
    \endfoot    
    \hline
    \endlastfoot
    
    Q-01 & 2841 & 2789 & 3147 & 2519 & 2609 & 2550 & 1713 & 1662 & 1679 & 1728 \\
    \hline
    Q-02 & 3189 & 5668 & 5065 & 2833 & 3021 & 2831 & 1810 & 1950 & 1917 & 2059 \\
    \hline
    Q-03 & 3056 & 6123 & 5101 & 6958 & 2857 & 2636 & 1813 & 1951 & 1919 & 2004 \\
    \hline
    Q-04 & 3265 & 6223 & 4752 & 7841 & 3061 & 2848 & 0* & 2174 & 2011 & 2097 \\ 
    \hline
    Q-05 & 6386 & 6021 & 6859 & 5488 & 2627 & 5685 & 3870 & 3856 & 3850 & 3982 \\
    \hline
    Q-06 & 6307 & 6093 & 6849 & 5597 & 2664 & 5582 & 3912 & 3801 & 3803 & 3915 \\
    \hline
    Q-07 & 7178 & 6203 & 3927 & 5697 & 2993 & 2799 & 4197 & 3083 & 2210 & 2386 \\
    \hline
    Q-08 & 3003 & 2934 & 3252 & 2628 & 2621 & 2633 & 1831 & 1754 & 1764 & 1840 \\
    \hline
    Q-09 & 2894 & 2823 & 3243 & 7064 & 2621 & 2580 & 4297 & 1664 & 1673 & 1720 \\
    \hline
    Q-10 & 6505 & 6173 & 6946 & 5798 & 2877 & 5673 & 3988 & 3942 & 3922 & 4018 \\
    \hline
    Q-11 & 6574 & 6230 & 6972 & 5792 & 2826 & 5712 & 3998 & 3944 & 3920 & 4025 \\ 
    \hline
    Q-12 & 6566 & 6200 & 6925 & 5727 & 2466 & 5677 & 3973 & 3927 & 3965 & 4022 \\
    \hline
    Q-13 & 6369 & 6174 & 6928 & 5621 & 2727 & 5617 & 3916 & 3813 & 3807 & 3930 \\
    \hline
    Q-14 & 6044 & 5783 & 6605 & 5201 & 2843 & 2552 & 3508 & 1646 & 1646 & 1701 \\
    \hline
    Q-15 & 6055 & 5809 & 6697 & 5239 & 2658 & 2623 & 3533 & 3423 & 3417 & 3527 \\
    \hline
    Q-16 & 6094 & 5829 & 6655 & 5247 & 2696 & 5267 & 3550 & 3437 & 3438 & 3554 \\
    \hline
    Q-17 & 6152 & 5890 & 6709 & 5277 & 3117 & 5286 & 3566 & 3457 & 3457 & 3570 \\
    \hline
    Q-18 & 6142 & 5867 & 6721 & 5279 & 2868 & 5290 & 3569 & 3460 & 3460 & 3575 \\
    \hline
    Q-19 & 6146 & 5886 & 6685 & 5278 & 3117 & 5287 & 3565 & 3457 & 3457 & 3570 \\
    \hline
    Q-20 & 6187 & 5949 & 6724 & 20770 & 2859 & 2729 & 3693 & 3587 & 5374 & 3696 \\
    \hline
    Q-21 & 34865 & 34023 & 35594 & 21463 & 2950 & 5062 & 0* & 25882 & 28049 & 20108 \\
    \hline
    Q-22 & 34822 & 25803 & 35862 & 33235 & 2994 & 5426 & 3601 & 11173 & 26946 & 21859 \\
    \hline
    Q-23 & 6877 & 6191 & 6985 & 5551 & 2745 & 5562 & 3788 & 3678 & 3679 & 3791 \\
    \hline
    Q-24 & 17319 & 12892 & 19398 & 19867 & 3021 & 5180 & 3638 & 11612 & 15648 & 11163 \\
    \hline
    Q-25 & 84066 & 113426 & 87740 & 84946 & 3065 & 2810 & 3650 & 55193 & 12960 & 44105 \\
\end{longtable}

%\end{landscape}
